# Supplementary material for: Electron correlations rule the phonon-driven instability in single layer TiSe$_2$
Source: arXiv:2203.10658 ancillary file (2022-12-09)
Supplement: Supplementary file 1 [file tise2_sm.pdf]

# Supplemental Material:
# Electron correlations rule phonon-driven instability in single layer $TiSe_2$

Dino Novko,[1,2,*] Zahra Torbatian,[3] and Ivor Lončarić[4]

[1] *Institute of Physics, 10000 Zagreb, Croatia*

[2] *Donostia International Physics Center (DIPC), 20018 Donostia-San Sebastián, Spain*

[3] *School of Nano Science, Institute for Research in Fundamental Sciences (IPM), 19395-5531 Tehran, Iran*

[4] *Ruđer Bošković Institute, 10000 Zagreb, Croatia*

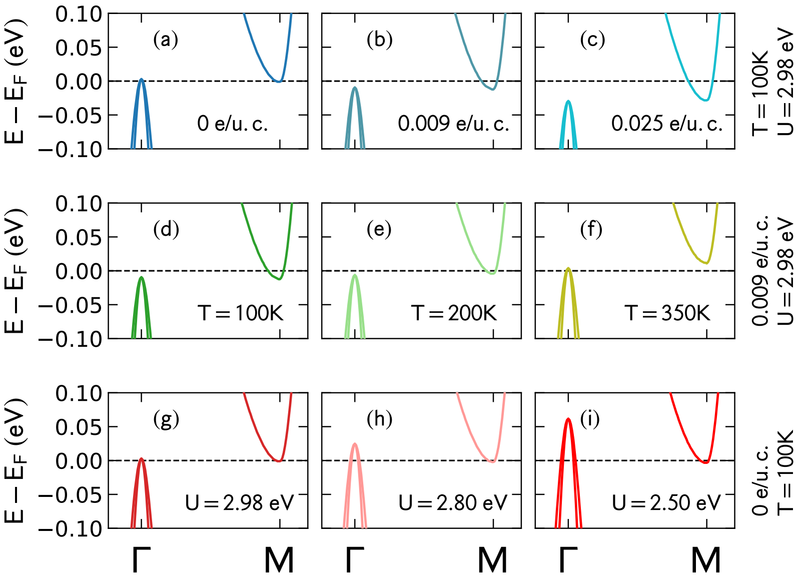


FIG. S1. Electronic band structure of single layer $TiSe_2$ in the original $1 \times 1$ unit cell as obtained with PBE+U calculated for (a)-(c) different electron-doping concentrations with $T = 100\,\mathrm{K}$ and $U = 2.98\,\mathrm{eV}$, (d)-(f) three different electron temperatures with $x = 0.009\,e^-/\mathrm{u.c.}$ and $U = 2.98\,\mathrm{eV}$, as well as for (g)-(i) three Hubbard parameters with $x = 0\,e^-/\mathrm{u.c.}$ and $T = 100\,\mathrm{K}$.

* dino.novko@gmail.com

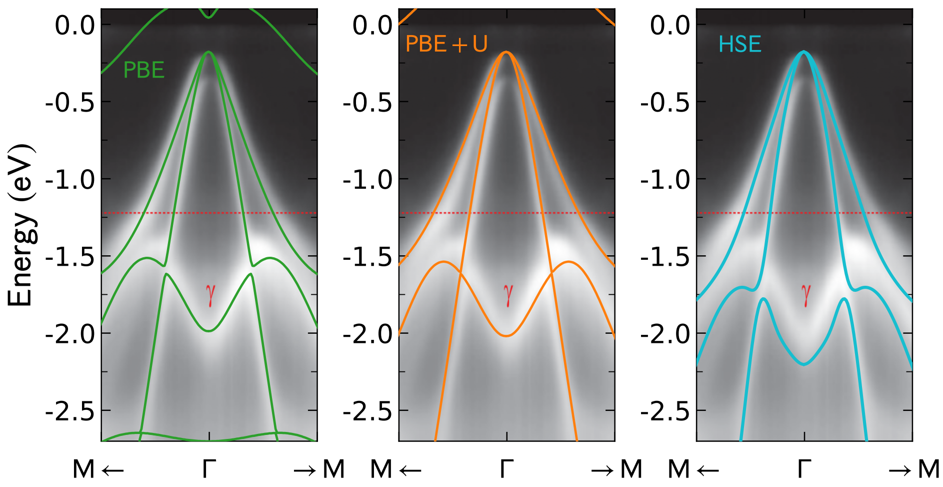


FIG. S2. Electronic band structure of single layer $TiSe_2$ in the original $1 \times 1$ unit cell as obtained with (left) PBE, (middle) PBE+U, and (right) HSE06 [S1]. The calculated results are compared with experimental ones [S2]. The bandwidth of the Se-$p_{x,y}$ states and the position of the Se-$p_z$ state (marked with the red $\gamma$) are well described with PBE and PBE+U, while not so well with HSE. The PBE results have, however, problem of the large negative indirect band gap between the Γ and M points of the BZ, which is fixed with the PBE+U approach.

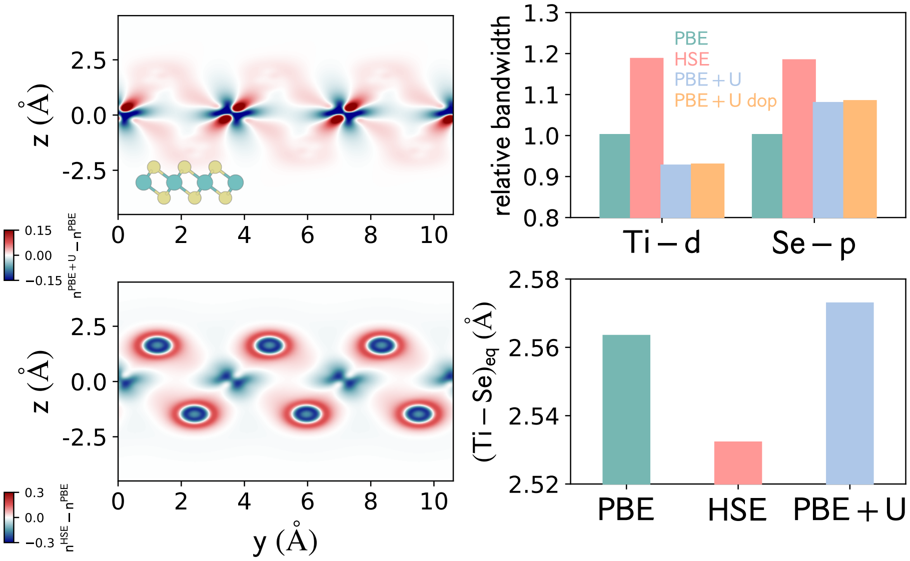


FIG. S3. Comparison between the electronic structures of the $TiSe_2$ as obtained with PBE, PBE+U and HSE. Left panels show the relative change of the charge distributions when PBE is substituted with PBE+U (upper left) and HSE (lower left). The upper right panel show the relative bandwidths of the relevant states in $TiSe_2$ (i.e., relative to the PBE result), and the lower right panel shows bond lengths between the Ti and Se atoms when PBE, HSE, and PBE+U are employed. PBE+U result compared to PBE tends to distribute more charge along the Ti-Se length and around Se atom since there is an additional on-site repulsion for the Ti-$d$ orbitals. In accordance to that, the Hubbard interaction will tend to increase the bond length between Ti and Se atoms, therefore reducing the electron-phonon coupling of the CDW mode. The hybrid HSE functional acts in the opposite way, that is, the distribution of charge compared to PBE introduces more polarization, and correspondingly the length of the Ti-Se bond is reduced. Regarding the bandwidth and the localization of the Ti-$d$ states, we observe that the increase of the bandwidth and delocalization (the HSE case) results in the larger Kohn anomaly, larger electron-phonon coupling strength of the relevant CDW mode, and higher $T_{CDW}$. See similar conclusions drawn in Ref. [S3] for $NbSe_2$ and $NbS_2$.

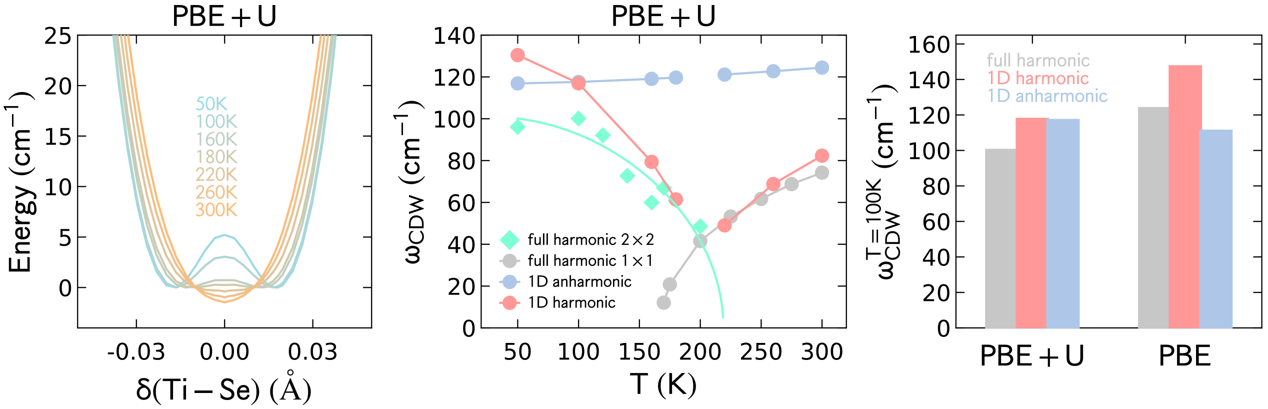


FIG. S4. (Left) 1D potential energy surface $V_{1D}(q)$ for the CDW amplitude motion (see the atomic displacements below in Fig. S5) as a function of the Ti-Se bond length modification ($q$) and for the PBE+U functional. The results are shown for different values of the electronic temperature. The time-independent Schrödinger $H_{1D}\phi_n = E_n\phi_n$ $[H_{1D} = -\hbar/2m_{\text{eff}}(\partial^2/\partial q^2) + V_{1D}(q)]$ is solved for each of these 1D potentials (i.e., for each temperature) by using the 1D discrete variable representation (DVR) of the kinetic part [S4, S5]. For the effective mass we use $m_{\text{eff}} = 328288$ a.u., which corresponds to six times the reduced mass of Ti and Se atoms (six bond lengths involved in CDW amplitude motion in the 2×2 cell). However, the results turn out to be quite robust with respect to the different choices of the mass parameter. See also Ref. S6 regarding difficulties in determining the effective mass of the relevent phonon mode. (Middle) Blue dots are the results of the diagonalization of the 1D potential energy curves presented in the left panel (anharmonic results). We also show the harmonic results as obtained from the effective harmonic potentials fitted to the minima of the 1D potential energy curves (red dots). These results are compared to our harmonic DFPT results as presented in the main text (green and grey). (Right) Frequencies of the amplitude mode for T = 100K as obtained with PBE+U and PBE. In grey we show harmonic DFPT results as obtained in the main text, and in blue (red) we show the anharmonic (harmonic) results from the 1D potential energy curves. Anharmonic corrections turn out to be larger for the PBE functional. This could be expected if one considers that if the phonon frequencies are modified over a larger region of the BZ, the phonon entropy is more important [S7, S8]. Namely, the Kohn anomaly is larger in the case of PBE compared to PBE+U.

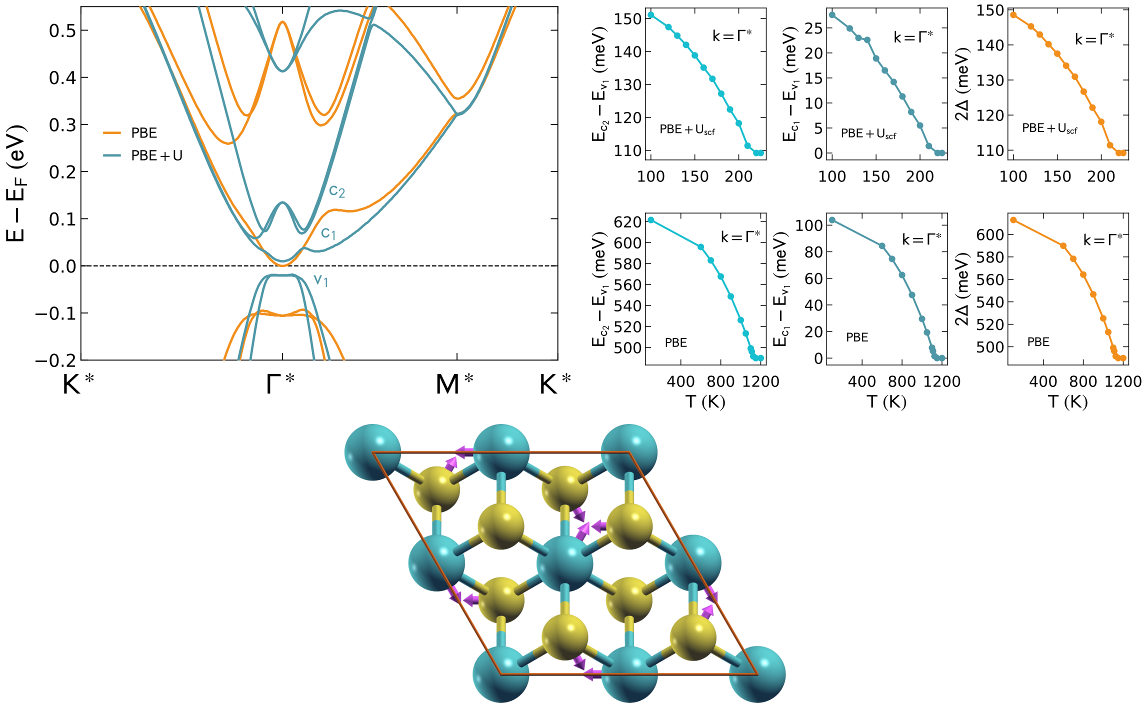


FIG. S5. (Upper left) Electronic band structure of single layer $TiSe_2$ in the CDW $2\times2$ supercell as obtained with PBE (orange) and PBE+U (blue). (Upper right) The corresponding energy gaps at $k = \Gamma^*$ between first valence band and second conduction band ($E_{c_2} - E_{v_1}$), as well as between first valence band and first conduction band ($E_{c_1} - E_{v_1}$). The CDW order parameter $\Delta$ is calculated as $E_{c_2} - E_{v_1} = \sqrt{(E_{c_1} - E_{v_1})^2 + (2\Delta)^2}$. (Below) The atomic displacements in the CDW $2 \times 2$ supercell. These characteristic pattern of displacement is formed from the phonon eigenvectors of the CDW mode at the three non-equivalent $\overline{\mathrm{M}}$ points. Please note that here the Se atoms are relaxed for each temperature with PBE+U also in the z direction. Therefore, the $T_{\mathrm{CDW}}$ obtained with PBE+U are a bit higher than the corresponding temperature obtained with DFPT for $1 \times 1$ cell (as presented in the main text), where we relaxed the Se atoms with PBE for $T \gg T_{\mathrm{CDW}}$ and we kept it fixed while changing the temperature.

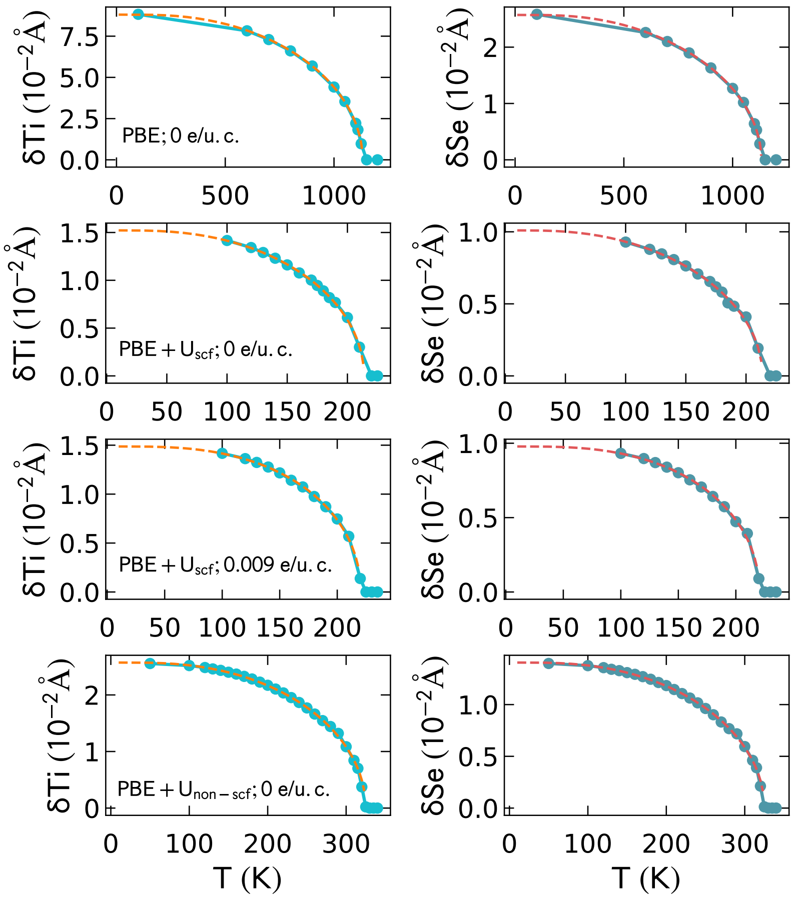


FIG. S6. Periodic lattice displacements for Ti and Se atoms in the CDW 2×2 supercell (i.e., distortions of Ti and Se atoms along the directions shown in Fig. S5) as obtained with PBE and PBE+U. The results are depicted for self-consistently obtained Hubbard parameter $U_{scf} = 2.98\,eV$, for arbitrarily chosen parameter $U_{non-scf} = 2.5\,eV$, as well as for finite electron doping $x = 0.009\,e^-/u.c.$ The distortions represent the equilibrium positions of atoms for each of the temperature. Please note that here the Se atoms are relaxed for each temperature with PBE+U also in the z direction. Therefore, the $T_{CDW}$ obtained with PBE+U are a bit higher than the corresponding temperature obtained with DFPT for $1 \times 1$ cell (as presented in the main text), where we relaxed the Se atoms with PBE for $T \gg T_{CDW}$ and we kept it fixed while changing the temperature. The dashed lines are corresponding fits to the following function $a\tanh(b\sqrt{c/T-1})$.

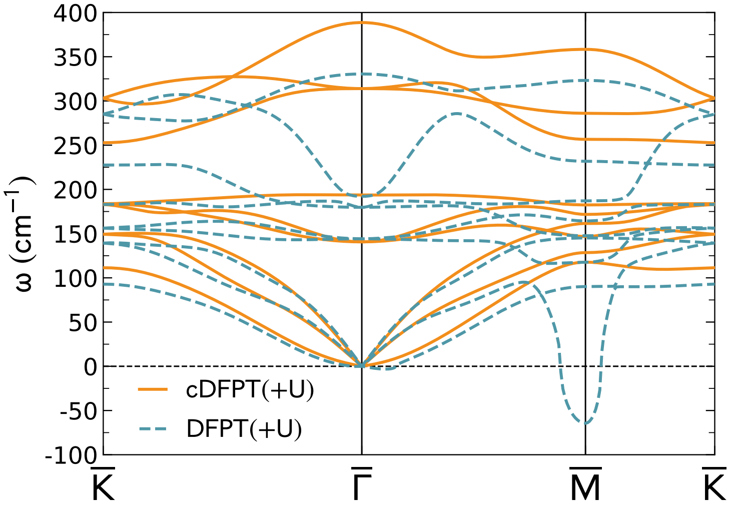


FIG. S7. Phonon band structure of single layer $TiSe_2$ in the original $1 \times 1$ unit cell as obtained with normal and constrained density functional perturbation theories (i.e., DFPT and cDFPT). In both cases Hubbard correction is used $U_{scf} = 2.98\,eV$. Within the current cDFPT calculation we have restricted intraband and interband electron transitions between two Se-$p$ highest valence states at Γ and one Ti-$d$ state at M, which are obviously the most important for the Kohn anomaly at the $\overline{M}$ point of the BZ.

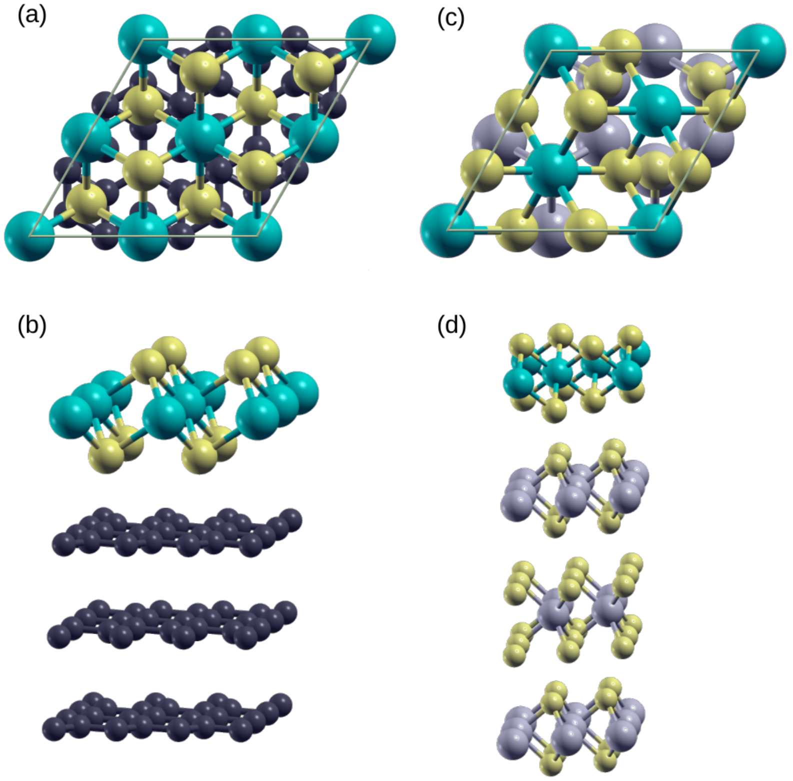


FIG. S8. Top and side views of $TiSe_2$ adsorbed on (a)-(b) graphite and (c)-(d) $MoS_2$ surfaces, which are both simulated with 3 layers. In each cases the structure of $TiSe_2$ is kept as in free-standing case, while the surface unit cell is modified accordingly.

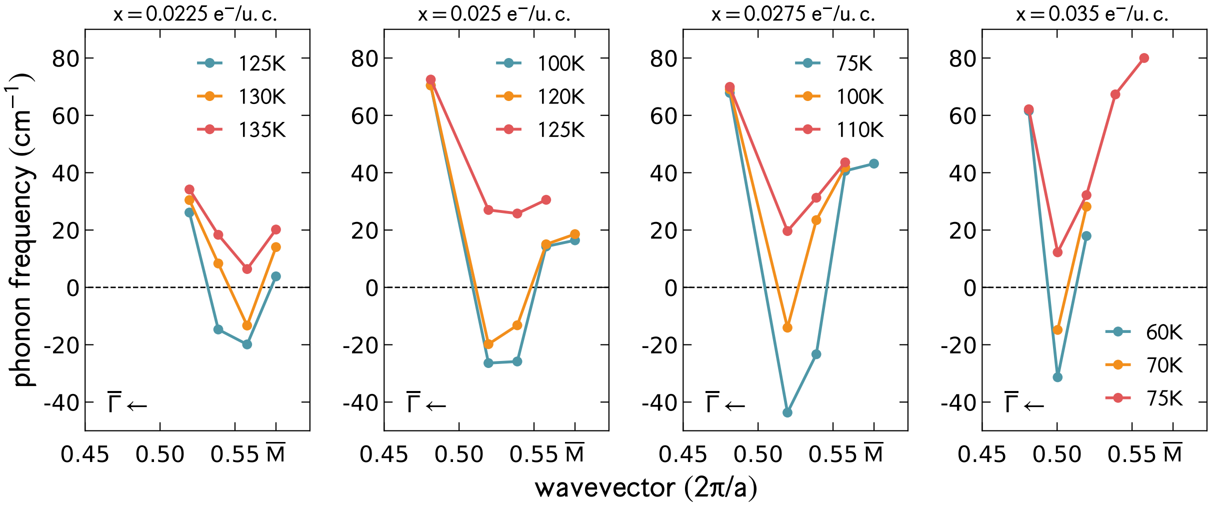


FIG. S9. Phonon frequencies of the acoustic $A_{1u}$ (CDW) phonon mode in the vicinity of the $\overline{\mathrm{M}}$ point of the BZ as a function of electron excess charge and temperature obtained with PBE+U. For dopings approximately higher than $0.02\,e^-$/u.c. the CDW phonon mode at the $\mathbf{q} = \overline{\mathrm{M}}$ becomes stable for certain temperatures, while at $\mathbf{q} < \overline{\mathrm{M}}$ it remains unstable. In that case, the CDW is incommensurate with periodicity much larger than $2 \times 2$.

## S1. CONSTRAINED DENSITY FUNCTIONAL PERTURBATION THEORY

Within the density functional perturbation theory (DFPT) [S9], the dynamical matrix is defined as

$$\mathcal{D}(\mathbf{q},\omega) = \int d\mathbf{r}\Delta n(\mathbf{r};\mathbf{q},\omega)\Delta V_{\mathrm{ion}}(\mathbf{r}) + \int d\mathbf{r}n(\mathbf{r})\Delta^2 V_{\mathrm{ion}}(\mathbf{r}), \tag{S1}$$

where the perturbation of the charge density with the displacement has the following form within the linear response

$$\Delta n(\mathbf{r};\mathbf{q},\omega) = \sum_{\mu\mu'\mathbf{k}} \frac{[f(\varepsilon_{\mu\mathbf{k}}) - f(\varepsilon_{\mu'\mathbf{k}+\mathbf{q}})]d^*_{\mu\mu',\nu}(\mathbf{k},\mathbf{q},\omega)}{\omega + i\eta + \varepsilon_{\mu\mathbf{k}} - \varepsilon_{\mu'\mathbf{k}+\mathbf{q}}}\psi^*_{\mu\mathbf{k}}(\mathbf{r})\psi_{\mu'\mathbf{k}+\mathbf{q}}(\mathbf{r}). \tag{S2}$$

The screened deformation potential is defined as $d^*_{\mu\mu',\nu}(\mathbf{k},\mathbf{q},\omega) = \langle\psi_{\mu'\mathbf{k}+\mathbf{q}}|\,\Delta_{\mathbf{q}\nu}V_{\mathrm{scf}}(\mathbf{r},\omega)\,|\psi_{\mu\mathbf{k}}\rangle$. The self-consistent potential is $\Delta_{\mathbf{q}\nu}V_{\mathrm{scf}}(\mathbf{r},\omega) = \Delta_{\mathbf{q}\nu}V_{\mathrm{ion}}(\mathbf{r}) + \int d\mathbf{r}'K(\mathbf{r},\mathbf{r}')\Delta_{\mathbf{q}\nu}n(\mathbf{r}',\omega)$ [where $K(\mathbf{r},\mathbf{r}') = \delta E_{Hxc}[n]/\delta n(\mathbf{r})\delta n(\mathbf{r}')$]. The prefactor $1/N_{\mathbf{k}}$ is assumed everywhere in front of $\mathbf{k}$ summations. Note that the dynamical screening is usually approximated with the static one, i.e., $\Delta_{\mathbf{q}\nu}V_{\mathrm{scf}}(\omega) \to \Delta_{\mathbf{q}\nu}V_{\mathrm{scf}}(0)$ [S10]. By introducing Eq. (S2) into Eq. (S1), the force constant matrix becomes

$$\mathcal{D}(\mathbf{q},\omega) = \sum_{\mu\mu'\mathbf{k}} \frac{[f(\varepsilon_{\mu\mathbf{k}}) - f(\varepsilon_{\mu'\mathbf{k}+\mathbf{q}})]d^*_{\mu\mu',\nu}(\mathbf{k},\mathbf{q},\omega)d^b_{\mu\mu',\nu}(\mathbf{k},\mathbf{q})}{\omega + i\eta + \varepsilon_{\mu\mathbf{k}} - \varepsilon_{\mu'\mathbf{k}+\mathbf{q}}} + \int d\mathbf{r}n(\mathbf{r})\Delta^2 V_{\mathrm{ion}}(\mathbf{r}), \tag{S3}$$

where $d^b_{\mu\mu',\nu}(\mathbf{k},\mathbf{q}) = \langle\psi_{\mu'\mathbf{k}+\mathbf{q}}|\,\Delta_{\mathbf{q}\nu}V_{\mathrm{ion}}(\mathbf{r})\,|\psi_{\mu\mathbf{k}}\rangle$ is the bare deformation potential. Note that Eq. (S3) is usually expressed in the form where $d^b_{\mu\mu',\nu}(\mathbf{k},\mathbf{q})$ is replaced with $d_{\mu\mu',\nu}(\mathbf{k},\mathbf{q},\omega)$ by using the following equation $\Delta V_{\mathrm{ion}}(\mathbf{r}) = \Delta V_{\mathrm{scf}}(\mathbf{r},\omega) - \int d\mathbf{r}'K(\mathbf{r},\mathbf{r}')\Delta n(\mathbf{r}',\omega)$. In the standard DFPT, the adiabatic phonon energies $\omega_{\mathrm{A}}$ are obtained as $\omega^2_{\mathrm{A}} = \mathcal{D}(\mathbf{q},0)/M$:

$$\omega^2_{\mathrm{A}} = \frac{1}{M}\sum_{\mu\mu'\mathbf{k}} d^*_{\mu\mu',\nu}(\mathbf{k},\mathbf{q})d^b_{\mu\mu',\nu}(\mathbf{k},\mathbf{q})\frac{f(\varepsilon_{\mu\mathbf{k}}) - f(\varepsilon_{\mu'\mathbf{k}+\mathbf{q}})}{\varepsilon_{\mu\mathbf{k}} - \varepsilon_{\mu'\mathbf{k}+\mathbf{q}}} + \frac{1}{M}\int d\mathbf{r}n(\mathbf{r})\Delta^2 V_{\mathrm{ion}}(\mathbf{r}), \tag{S4}$$

where we define $d^*_{\mu\mu',\nu}(\mathbf{k},\mathbf{q}) \equiv d^*_{\mu\mu',\nu}(\mathbf{k},\mathbf{q},\omega = 0)$. Now it is possible to study the impact of selected relevant electronic transitions on the dynamical matrix and corresponding phonon modes by removing these transitions from the Sternheimer linear response equations [S9]. Such procedure for calculating partially renormalized phonon energies,

which include the screening effects coming from reduced number of electronic transitions, is described in Refs. [S11–S13]. Here we study the role of interband and intraband electron transitions including only the two highest valence Se-$p$ bands and first conduction Ti-$d$ band for the formation of the $\mathbf{q} = \overline{\mathrm{M}}$ Kohn anomaly. We simply name this subset of the three electron bands as $P$.

The partially renormalized adiabatic phonon energy for which the intraband and interband transitions within this $P$ subset are removed can be written as

$$(\omega_{\mathrm{A}}^{p})^2 = \frac{1}{M} \sum_{\mu \neq P, \mu' \neq P, \mathbf{k}} d^{*}_{\mu\mu',\nu}(\mathbf{k},\mathbf{q}) d^{b}_{\mu\mu',\nu}(\mathbf{k},\mathbf{q}) \frac{f(\varepsilon_{\mu\mathbf{k}}) - f(\varepsilon_{\mu'\mathbf{k}+\mathbf{q}})}{\varepsilon_{\mu\mathbf{k}} - \varepsilon_{\mu'\mathbf{k}+\mathbf{q}}} + \frac{1}{M} \int d\mathbf{r} n(\mathbf{r}) \Delta^2 V_{\mathrm{ion}}(\mathbf{r}). \tag{S5}$$

By subtracting partially [Eq. (S4)] from fully [Eq. (S5)] renormalized adiabatic phonon energy one gets

$$\omega_{\mathrm{A}}^2 - (\omega_{\mathrm{A}}^{p})^2 = \frac{1}{M} \sum_{\mu = P, \mu' = P, \mathbf{k}} d^{*}_{\mu\mu',\nu}(\mathbf{k},\mathbf{q}) d^{b}_{\mu\mu',\nu}(\mathbf{k},\mathbf{q}) \frac{f(\varepsilon_{\mu\mathbf{k}}) - f(\varepsilon_{\mu'\mathbf{k}+\mathbf{q}})}{\varepsilon_{\mu\mathbf{k}} - \varepsilon_{\mu'\mathbf{k}+\mathbf{q}}}, \tag{S6}$$

which corresponds to the partially-screened static phonon self-energy $\pi^{p}_{\nu}(\mathbf{q})$ (which includes only the effects from the intraband and interband transitions within the $P$ subset) if the expression Eq. (S6) is divided by $\omega_{\mathrm{A}}^{p}$, i.e.,

$$\frac{\omega_{\mathrm{A}}^2 - (\omega_{\mathrm{A}}^{p})^2}{2\omega_{\mathrm{A}}^{p}} = \frac{1}{2M\omega_{\mathrm{A}}^{p}} \sum_{\mu = P, \mu' = P, \mathbf{k}} d^{*}_{\mu\mu',\nu}(\mathbf{k},\mathbf{q}) d^{b}_{\mu\mu',\nu}(\mathbf{k},\mathbf{q}) \frac{f(\varepsilon_{\mu\mathbf{k}}) - f(\varepsilon_{\mu'\mathbf{k}+\mathbf{q}})}{\varepsilon_{\mu\mathbf{k}} - \varepsilon_{\mu'\mathbf{k}+\mathbf{q}}}, \tag{S7}$$

or if the screened and bare electron-phonon coupling functions are defined as $g_{\mu\mu',\nu}(\mathbf{k},\mathbf{q}) = \langle\psi_{\mu\mathbf{k}}|\, \Delta_{\mathbf{q}\nu} V_{\mathrm{scf}}(\omega = 0)\, |\psi_{\mu'\mathbf{k}+\mathbf{q}}\rangle / \sqrt{2M\omega_{\mathrm{A}}^{p}}$ and $g^{b}_{\mu\mu',\nu}(\mathbf{k},\mathbf{q}) = \langle\psi_{\mu\mathbf{k}}|\, \Delta_{\mathbf{q}\nu} V_{\mathrm{ion}}\, |\psi_{\mu'\mathbf{k}+\mathbf{q}}\rangle / \sqrt{2M\omega_{\mathrm{A}}^{p}}$, respectively, we finally have

$$\frac{\omega_{\mathrm{A}}^2 - (\omega_{\mathrm{A}}^{p})^2}{2\omega_{\mathrm{A}}^{p}} = \sum_{\mu = P, \mu' = P, \mathbf{k}} g^{*}_{\mu\mu',\nu}(\mathbf{k},\mathbf{q}) g^{b}_{\mu\mu',\nu}(\mathbf{k},\mathbf{q}) \frac{f(\varepsilon_{\mu\mathbf{k}}) - f(\varepsilon_{\mu'\mathbf{k}+\mathbf{q}})}{\varepsilon_{\mu\mathbf{k}} - \varepsilon_{\mu'\mathbf{k}+\mathbf{q}}} \equiv \pi^{p}_{\nu}(\mathbf{q}). \tag{S8}$$

Therefore, by calculating $\omega_A$ and $\omega_A^p$ using DFPT and cDFPT one can extract the momemntum-dependent static phonon self-energy $\pi^{p}_{\nu}(\mathbf{q})$. The corresponding results for 1L $TiSe_2$ are presented in Fig. S7.

Furthermore, by simplifying $g^{*}_{\mu\mu',\nu}(\mathbf{k},\mathbf{q}) g^{b}_{\mu\mu',\nu}(\mathbf{k},\mathbf{q}) \approx |g_{\mu\mu',\nu}(\mathbf{k},\mathbf{q})|^2 \approx |g_{\nu}(\mathbf{q})|^2$, the static phonon self-energy can be written via the charge correlation function $\chi^0(\mathbf{q})$ as

$$\pi^{p}_{\nu}(\mathbf{q}) \approx |g_{\nu}(\mathbf{q})|^2 \sum_{\mu = P, \mu' = P, \mathbf{k}} \frac{f(\varepsilon_{\mu\mathbf{k}}) - f(\varepsilon_{\mu'\mathbf{k}+\mathbf{q}})}{\varepsilon_{\mu\mathbf{k}} - \varepsilon_{\mu'\mathbf{k}+\mathbf{q}}} \equiv |g_{\nu}(\mathbf{q})|^2 \chi^0(\mathbf{q}). \tag{S9}$$

This allows for disentanglement of the purely electron contributions (as in Peierls instability) coming from $\chi^0(\mathbf{q})$ and the electron-phonon contributions coming from the effective coupling $|g_{\nu}(\mathbf{q})|^2$.

Here we would like to note that Hubbard on-site corrections enter cDFPT in the very same manner as the U enters standard DFPT, i.e., via change of the Hubbard potential that enters the variation of the total Kohn-Sham potential (Eq. (2) in Ref. S14) and second derivative of Hubbard energy correction (Eq. (4) in Ref. S14) as part of the total dynamical matrix. That is, the difference in the DFPT+U and cDFPT+U is not in the expressions, but in the number of the states included in the screening of the phonons.

## S2. COMPUTATIONAL DETAILS

The ground-state calculations of 1L $TiSe_2$ were done by means of the QUANTUM ESPRESSO (QE) package [S15] with a plane-wave cutoff energy of 80 Ry. Optimized norm-conserving Vanderbilt pseudopotentials [S16] were used with the PBE exchange-correlation functional [S17]. To improve the electronic band structure the on-site Hubbard correction to the DFT was used [S18]. Hubbard U was calculated from first principles by employing the self-consistent linear approach [S19], where we iterate calculations of the Hubbard parameters and the corresponding structural optimization until we reach the satisfactory convergence [S20]. Momentum mesh needed for calculating U was set to $\mathbf{q} = 6 \times 6 \times 1$, while convergence threshold for the corresponding response matrix was set to $10^{-8}$ Ry. The atomic orbitals (read from pseudopotential) are used to build the Hubbard projectors. For the undoped 1L $TiSe_2$ we obtained

$U_{scf} = 2.977\,eV$. The self-consistent *ab initio* calculations of U for Ti atom was also calculated for the two cases where $TiSe_2$ is adsorbed on 3L-graphite and 3L-$MoS_2$ (see Fig. S8). In both cases the atomic configuration of $TiSe_2$ is as in the case of the free-standing monolayer, while the surfaces are modified accordingly. In Ref. S21 it was argued that Hubbard parameter U is position dependent and that it needs to be calculated for distorted atoms in the CDW phase in order to get accurate results. We have therefore also calculated U for the Ti atoms in distorted $2 \times 2$ cell. In that case there are two nonequivalent Ti atoms (one in its initial position and other distorted by amount presented in Fig. S6), and we obtain $U_{scf} = 3.00\,eV$ and $U_{scf} = 3.02\,eV$, respectively. These variations in Hubbard parameter are insignificant and not enough to produce some modifications to the transition temperature and other CDW properties. In addition, the monolayer-surface distance is optimized with the vdW-DF-cx functional [S22], to properly account for the van der Waals interactions. For $TiSe_2$ on surface the $\mathbf{q}$-momentum mesh needed for calculating U was set to $3 \times 3 \times 1$, while convergence threshold to $10^{-7}$ Ry. A Monkhorst-Pack grid from $48 \times 48 \times 1$ to $120 \times 120 \times 1$ was used for sampling the Brillouin zone. The Fermi-Dirac smearing functions were used with $T = 100 - 1400\,K$. A lattice parameter $a = 3.537\,Å$ and a vacuum space of $18.5\,Å$ were adopted (structural optimization with PBE+U gives us $a = 3.62\,Å$ and $U_{scf} = 2.96\,eV$, but we instead use the PBE lattice parameter, since it provides better electronic structure and the value perfectly agrees with the experimental). Relaxation of the Se atoms within the unit cell is performed with PBE functional. The atomic positions are relaxed until the forces are less than $10^{-6}\,Ry/a_0$ ($2.57 \times 10^{-5}\,eV/Å$). Electron and hole dopings were simulated by adding and removing, respectively, the electrons and introducing the compensating homogeneous charged background.

Phonon dynamics were simulated by using DFPT [S9] as well as DFPT corrected with Hubbard on-site interactions [S14, S19, S23], as implemented in QE. All phonon DFPT calculations for $1 \times 1$ structure presented in the main text were done with $\mathbf{k} = 96 \times 96 \times 1$, which was additionally checked to be well converged (see the brown stars in Fig. 1(d) of the main text). We note that dense $\mathbf{k}$ grids are important to obtain the right phonon instabilities with DFPT+U, since the Fermi surface of $TiSe_2$ is quite small. The phonon calculations of the CDW structure (aqua diamonds in Fig. 1(d) of the main text) are done on $2 \times 2$ structure with PLDs corresponding to each chosen temperature, which are taken from the relaxation calculations presented in Fig. S6. The corresponding momentum grid for the phonon calculations of the CDW structure were $\mathbf{k} = 48 \times 48 \times 1$. One could argue that since PBE+U opens a gap in $TiSe_2$ the nonanalytic term to the dynmical matrix, which accounts for the coupling of longitudinal vibrations with the macroscopic electric field, becomes relevant, and calculations of the Born effective charges and high-frequency dielectric functions are necessary [S14, S24–S26]. However, these corrections only apply for the long-wavelength part of the phonon momentum space, and therefore are not relevant for the CDW soft mode at the M point of the BZ. For the low-$T$ $2 \times 2$ structure the M soft phonon is folded to the center of the BZ, however, the $q \to 0$ limit in 2D, relevant for the present study, should not be affected by this coupling to the macroscopic electric field [S27]. Also, for the cases of electron-doped $TiSe_2$ it is clear that this coupling anyway becomes unimportant.

The charge correlation functions presented in the main text were calculated on the $\mathbf{k} = 96 \times 96 \times 1$ momentum grid, and restricted to the interband and intraband electron transitions including only the two highest valence Se-$p$ bands and first conduction Ti-$d$ band (i.e., the same restriction used in cDFPT calculations as explained in Sec. S1).

Calculations of the effective deformation potential $|D_\nu(\mathbf{q})|^2 = 2\omega_\nu |g_\nu(\mathbf{q})|^2$ presented in Fig. 2(e) of the main text with orange squares are obtained with the standard DFPT methods as implemented in QE in order to benchmark the effective EPC matrix elements extracted from cDFPT. The used momentum grid in that case was $\mathbf{k} = 96 \times 96 \times 1$, while broadening used for the double delta functions was 0.15 eV. The effective deformation potential can be obtained from phonon linewidths $\gamma_{\mathbf{q}\nu}$, i.e., from the EPC strength $\lambda_{\mathbf{q}\nu}$ as

$$|D_\nu(\mathbf{q})|^2 = 2\omega_{\mathbf{q}\nu} \frac{\sum_{\mu,\mu',\mathbf{k}} |g_\nu^{\mu\mu'}(\mathbf{k},\mathbf{q})|^2 \delta(\varepsilon_{\mu\mathbf{k}} - \varepsilon_F)\delta(\varepsilon_{\mu'\mathbf{k}+\mathbf{q}} - \varepsilon_F)}{\sum_{\mu,\mu',\mathbf{k}} \delta(\varepsilon_{\mu\mathbf{k}} - \varepsilon_F)\delta(\varepsilon_{\mu'\mathbf{k}+\mathbf{q}} - \varepsilon_F)}. \tag{S10}$$

The PBE results for $|D_\nu(\mathbf{q})|^2$ as obtained with cDFPT [solid orange line in Fig. 2(e) of the main text] is in a pretty good agreement with $|D_\nu(\mathbf{q})|^2$ as obtained from the standard DFPT according to Eq. (S10). Calculations of $\gamma_{\mathbf{q}\nu}$ and $\lambda_{\mathbf{q}\nu}$ within DFPT+U are not implemented thus far, therefore, we use an alternative approach, i.e., cDFPT and cDFPT+U as in Sec. S1.

## SUPPLEMENTAL REFERENCES

[S1] J. Heyd, G. E. Scuseria, and M. Ernzerhof, Hybrid functionals based on a screened coulomb potential, The Journal of Chemical Physics **118**, 8207 (2003).

[S2] T. Jia, S. N. Rebec, S. Tang, K. Xu, H. M. Sohail, M. Hashimoto, D. Lu, R. G. Moore, and Z.-X. Shen, Epitaxial growth of TiSe 2 /TiO 2 heterostructure, 2D Materials **6**, 011008 (2018).

[S3] Y. Zheng, X. Jiang, X.-X. Xue, X. Yao, J. Zeng, K.-Q. Chen, E. Wang, and Y. Feng, Nuclear quantum effects on the charge-density wave transition in nbx2 (x = s, se), Nano Letters **22**, 1858 (2022).

[S4] J. C. Tremblay, G. Füchsel, and P. Saalfrank, Excitation, relaxation, and quantum diffusion of co on copper, Phys. Rev. B **86**, 045438 (2012).

[S5] D. Novko, M. Blanco-Rey, and J. C. Tremblay, Intermode coupling drives the irreversible tautomerization in porphycene on copper(111) induced by scanning tunnelling microscopy, The Journal of Physical Chemistry Letters **8**, 1053 (2017).

[S6] T. Esswein and N. A. Spaldin, Ferroelectric, quantum paraelectric, or paraelectric? calculating the evolution from batio$_3$ to srtio$_3$ to ktao$_3$ using a single-particle quantum mechanical description of the ions, Phys. Rev. Research **4**, 033020 (2022).

[S7] W. L. McMillan, Microscopic model of charge-density waves in $2h-$Tase$_2$, Phys. Rev. B **16**, 643 (1977).

[S8] J. E. Inglesfield, Bonding and phase transitions in transition metal dichalcogenide layer compounds, Journal of Physics C: Solid State Physics **13**, 17 (1980).

[S9] S. Baroni, S. de Gironcoli, A. Dal Corso, and P. Giannozzi, Phonons and related crystal properties from density-functional perturbation theory, Rev. Mod. Phys. **73**, 515 (2001).

[S10] F. Giustino, Electron-phonon interactions from first principles, Rev. Mod. Phys. **89**, 015003 (2017).

[S11] Y. Nomura and R. Arita, Ab initio downfolding for electron-phonon-coupled systems: Constrained density-functional perturbation theory, Phys. Rev. B **92**, 245108 (2015).

[S12] D. Novko, Broken adiabaticity induced by lifshitz transition in mos$_2$ and ws$_2$ single layers, Communications Physics **3**, 1 (2020).

[S13] J. Berges, E. G. C. P. van Loon, A. Schobert, M. Rösner, and T. O. Wehling, Ab initio phonon self-energies and fluctuation diagnostics of phonon anomalies: Lattice instabilities from dirac pseudospin physics in transition metal dichalcogenides, Phys. Rev. B **101**, 155107 (2020).

[S14] A. Floris, S. de Gironcoli, E. K. U. Gross, and M. Cococcioni, Vibrational properties of mno and nio from dft + $u$-based density functional perturbation theory, Phys. Rev. B **84**, 161102 (2011).

[S15] P. Giannozzi, S. Baroni, N. Bonini, M. Calandra, R. Car, C. Cavazzoni, D. Ceresoli, G. L. Chiarotti, M. Cococcioni, I. Dabo, and *et al.*, Quantum espresso: a modular and open-source software project for quantum simulations of materials, Journal of Physics: Condensed Matter **21**, 395502 (2009).

[S16] D. R. Hamann, Optimized norm-conserving vanderbilt pseudopotentials, Phys. Rev. B **88**, 085117 (2013).

[S17] J. P. Perdew, K. Burke, and M. Ernzerhof, Generalized gradient approximation made simple, Phys. Rev. Lett. **77**, 3865 (1996).

[S18] M. Cococcioni and S. de Gironcoli, Linear response approach to the calculation of the effective interaction parameters in the LDA + U method, Phys. Rev. B **71**, 035105 (2005).

[S19] I. Timrov, N. Marzari, and M. Cococcioni, Hubbard parameters from density-functional perturbation theory, Phys. Rev. B **98**, 085127 (2018).

[S20] I. Timrov, N. Marzari, and M. Cococcioni, Self-consistent hubbard parameters from density-functional perturbation theory in the ultrasoft and projector-augmented wave formulations, Phys. Rev. B **103**, 045141 (2021).

[S21] R. Bianco, M. Calandra, and F. Mauri, Electronic and vibrational properties of tise$_2$ in the charge-density-wave phase from first principles, Phys. Rev. B **92**, 094107 (2015).

[S22] K. Berland and P. Hyldgaard, Exchange functional that tests the robustness of the plasmon description of the van der waals density functional, Phys. Rev. B **89**, 035412 (2014).

[S23] A. Floris, I. Timrov, B. Himmetoglu, N. Marzari, S. de Gironcoli, and M. Cococcioni, Hubbard-corrected density functional perturbation theory with ultrasoft pseudopotentials, Phys. Rev. B **101**, 064305 (2020).

[S24] P. Giannozzi, S. de Gironcoli, P. Pavone, and S. Baroni, Ab initio calculation of phonon dispersions in semiconductors, Phys. Rev. B **43**, 7231 (1991).

[S25] X. Gonze and C. Lee, Dynamical matrices, born effective charges, dielectric permittivity tensors, and interatomic force constants from density-functional perturbation theory, Phys. Rev. B **55**, 10355 (1997).

[S26] L. Wirtz, A. Rubio, R. A. de la Concha, and A. Loiseau, Ab initio calculations of the lattice dynamics of boron nitride nanotubes, Phys. Rev. B **68**, 045425 (2003).

[S27] T. Sohier, M. Gibertini, M. Calandra, F. Mauri, and N. Marzari, Breakdown of optical phonons' splitting in two-dimensional materials, Nano Letters **17**, 3758 (2017).
